# Supplementary material for: Better Language Models of Code through Self-Improvement
Source: arXiv:2304.01228 source file (2023-05-10)
Supplement: Supplementary file 1 [file appendix_b.tex]

\section{Effect of $\theta_{fine-tuned}$ performance on gained improvement by $\theta_{improved}$}
\label{sec:appendix_b}
% \input{figures/plot}
% \begin{table} [t]
% \captionsetup{font=scriptsize}
% %\begin{center}
% \centering
% \resizebox{\linewidth}{!}{
%\begin{tabular}{p{12cm}p{7cm}}
%\begin{minipage}{0.75\textwidth}
%\resizebox{\textwidth}{!}{

\begin{table*} [t]
\begin{center}
\resizebox{0.99\textwidth}{!}{
\begin{tabular}{p{12cm}p{7cm}}
\begin{minipage}{0.75\textwidth}
\resizebox{\textwidth}{!}{

\begin{tabular}{lc c c c c c c c     c c c c c c c c c c c c}
\toprule
\multirow{2}{*}{Metrics} & \multicolumn{6}{c}{UniXCoder} & \multicolumn{6}{c}{CodeBERT} & \multicolumn{6}{c}{CodeT5} \\ 
\cmidrule(lr){2-7}\cmidrule(lr){8-13}\cmidrule(lr){14-20}
& Ruby & Javascript & Go & Python & Java & PHP & Ruby & Javascript & Go & Python & Java & PHP & Ruby & Javascript & Go & Python & Java & PHP \\
\midrule
    $r_1$ & -0.09 & 0.45 & 0.36 & 0.46 & 0.74 & 1.76 & 0.18 & 1.05 & 0.43 & 0.62 & 0.8 & 1.62 & 0.49 & 0.61 & 0.38 & 0.56 & 0.39 & 0.77 \\
\midrule
         $r_{2,1}$ & 0.53 & 0.44 & 0.47 & 0.47 & 0.67 & 1.06 & 0.36 & 0.71 & 0.94 & 0.62 & 0.69 & 1.02 & 0.66 & 0.65 & 0.55 & 0.5 & 0.38 & 0.92 \\
\cdashline{1-20}
         $r_{2,5}$ & 0.2 & 0.02 & 0.21 & 0.3 & 0.27 & 0.24 & 0.24 & 0.65 & 0.57 & 0.41 & 0.51 & 0.36 & 0.37 & 0.33 & 0.31 & 0.17 & 0.18 & 0.35 \\
\cdashline{1-20}
         $r_{2,10}$ & 0.63 & 0.12 & 0.42 & 0.44 & 0.33 & -0.06 & 0.3 & 0.61 & 0.65 & 0.41 & 0.5 & 0.22 & 0.41 & 0.29 & 0.33 & 0.16 & 0.19 & 0.48 \\

\bottomrule
\end{tabular}
}

\end{minipage}
\end{tabular}
}
\captionsetup{type=table}
\vspace{-0.5em}  
\caption{
    Reported values for $r_1$ and $r_{2,k}$ for $k \in {1, 5, 10}$
    % calculated by Equation~\ref{eq:r1_r2} and Equation~\ref{eq:r1_r2}
    for CodeT5, CodeBERT, and UniXCoder for code summarization across 6 languages.
}\label{table:r1_r2}
\end{center}
\vspace{-1em}
\end{table*}

\begin{table*} [t]
\begin{center}
\resizebox{0.99\textwidth}{!}{
\begin{tabular}{p{12cm}p{7cm}}
\begin{minipage}{0.75\textwidth}
\resizebox{\textwidth}{!}{
\begin{tabular}{lc c c lc c c c c cc}
\toprule
Models & Stages & Ruby & JavaScript & Go & Python & Java & PHP & Concode \\
\midrule
    CodeT5 & $P_{\theta_{fine-tuned}}(y=\hat{y_i} \mid x_i)$ & 1.45\% & 1.63\% & 3.22\% & 2.41\% & 4.02\% & 3.45\% & 33.56\% \\
       % & $P_{\theta_{improved}}(y=\hat{y_i} \mid x_i)$       & 7.10\% & 21.06\% & 19.82\% & 20.97\% & 17.13\% & 24.70\% & 41.25\% \\
       & $P_{\theta_{improved}}(y=\hat{y_i} \mid x_i)$       &\textbf{7.10\%} & \textbf{21.06\%} & \textbf{19.82\%} & \textbf{20.97\%} & \textbf{17.13\%} & \textbf{24.70\%} & \textbf{41.25\%} \\
       %&          & Our (multi-languages) & \textbf{} & \textbf{} & \textbf{} & \textbf{} & \textbf{} & \textbf{} & \textbf{} \\
% \cdashline{2-10}
%        & $PPL$    & Baseline          & 1.44 & 1.40 & 1.41 & 1.32 & 1.35 & 1.22 & 1.26 \\
%        &          & Our (specific language) & \textbf{1.59} & \textbf{1.63} & \textbf{1.65} & \textbf{1.50} & \textbf{1.47} & \textbf{1.31} & \textbf{1.31} \\
%        %&          & Our (multi-languages) & \textbf{} & \textbf{} & \textbf{} & \textbf{} & \textbf{} & \textbf{} & \textbf{} \\
\midrule
    CodeBERT & $P_{\theta_{fine-tuned}}(y=\hat{y_i} \mid x_i)$ & 0.33\% &  & 1.59\% & 1.61\% & 1.90\% & 3.52\% & - \\
       & $P_{\theta_{improved}}(y=\hat{y_i} \mid x_i)$ &  \textbf{1.52\%} & \textbf{7.73\%} & \textbf{10.65\%} & \textbf{13.90\%} & \textbf{7.86\%} & \textbf{14.26\%} & - \\
% \cdashline{2-10}
%          & $PPL$    & Baseline          & 78.11 & 368.89 & 15.97 & 22.97 & 24.24 & 16.96 & - \\
%          &          & Our      & \textbf{101.99} & \textbf{399.70} & \textbf{30.60} & \textbf{52.88} & \textbf{34.87} & \textbf{26.38} & - \\
\bottomrule
\end{tabular}
}

\end{minipage}
\end{tabular}
}
\captionsetup{type=table}
\vspace{-0.5em}  
\caption{
    Averaged probability of the greedy decoding generated sequences by $\theta_{fine-tuned}$ and $\theta_{improved}$ on test data for code summarization (CodeT5, CodeBERT) and code generation (CodeT5). The higher probability for each model is in bold.
}\label{table:seq_prob}
\end{center}
\vspace{-1em}
\end{table*}

This section extends the Discussion section to consider all value of $k \in \{1, 5, 10\}$
We investigate how gap in performance of $\theta_{fine-tuned}$ would affect the improvement gained by $\theta_{improved}$.
We choose code summarization as an demonstrated example and manipulate the numbers in Table~\ref{table:summarize} by the following logic
\begin{align}
    &r_1=s_{10,fined-tuned} - s_{1,fine-tuned} \\
    &r_{2,k} = s_{k,improved}-s_{k,fine-tuned}
\end{align}
where:
\begin{itemize}
\item $s_{i,j} =$ evaluation score (BLEU or CodeBLEU) on the test dataset. In which, $i$ denotes the beam size and $j$ denotes the model stage
\end{itemize}
	
In the above equations, $r_1$ can be understood as the gap of the score between beam size of 10 and 1 of $\theta_{fine-tuned}$ evaluated on the test dataset. 
And $r_{2,k}$ is the gap of the score evaluated with beam size of $k$ between $\theta_{improved}$ and $\theta_{fine-tuned}$ on the test dataset.

\begin{table} [t]
\captionsetup{}
\centering
\resizebox{\columnwidth}{!}{
\begin{tabular}{lc c c c c c}
\toprule
Beam sizes & $r$ & $R^2$ & least square equation \\ 
\midrule
1 & 0.77 & 0.592 & $y=0.362x+0.414$ \\
\midrule
5 & 0.27 &  0.072 & $y=0.090x+0.258$ & \\
\midrule
10 & -0.43 & 0.185 & $y=-0.177x+0.471$ & \\
\bottomrule
\end{tabular}
}

\vspace{-0.5em}  
\caption{
    Descriptive statistics for ($r_1$, $r_{2,k})$ for $k \in {1, 5, 10}$. $r$ represents pearson correlation, and $R^2$ represents coefficient of determination in linear regression.
    }\label{table:stats}
\vspace{-1em}
\end{table}

\begin{figure}
%\centering
%\resizebox{\linewidth}{!}{
 \centerline{\includegraphics[width=1\linewidth]{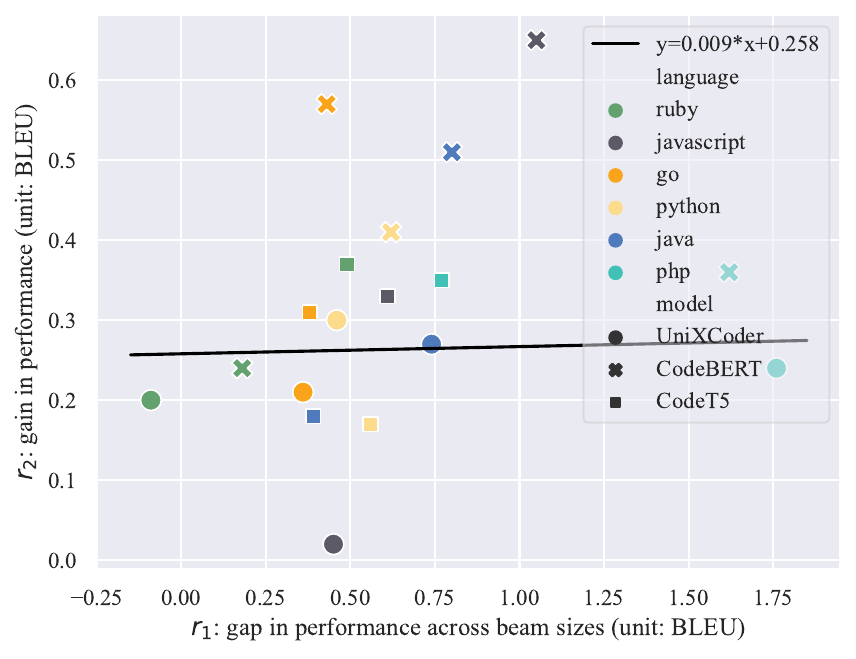}}
%}
\caption{
Scatter plot visualizing 
performance gap (in BLEU score) infered by different beam sizes (i.e 10 and 1) of $\theta_{fine-tuned}$
vs. 
performance gained (in BLEU score) by $\theta_{improved}$ infered with beam size of 5
}\label{figure:plot_5}
\vspace{-1em}
\end{figure}

\begin{figure}
%\centering
%\resizebox{\linewidth}{!}{
 \centerline{\includegraphics[width=1\linewidth]{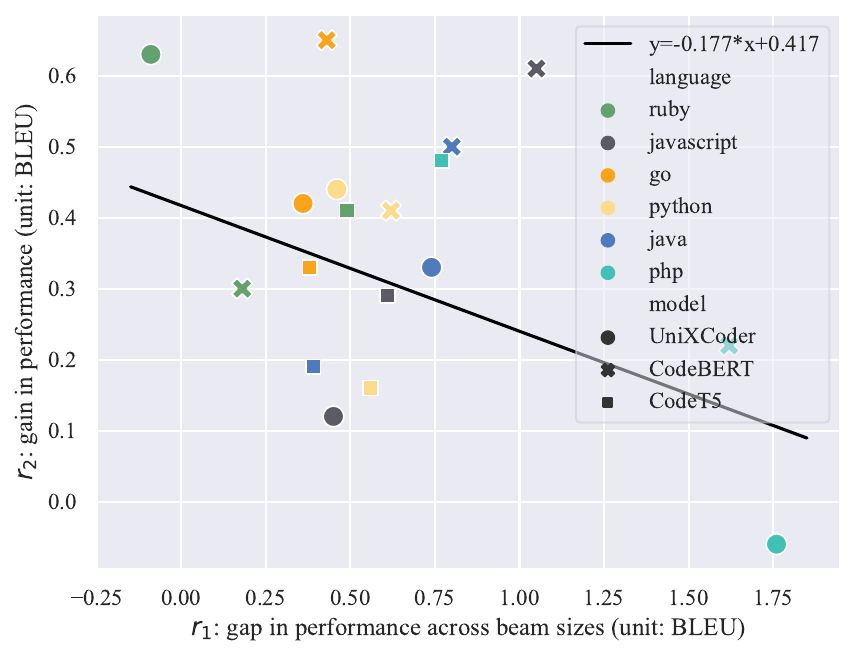}}
%}
\caption{
Scatter plot visualizing 
performance gap (in BLEU score) infered by different beam sizes (i.e 10 and 1) of $\theta_{fine-tuned}$
vs. 
performance gained (in BLEU score) by $\theta_{improved}$ infered with beam size of 10
}\label{figure:plot_10}
\vspace{-1em}
\end{figure}

The full statistics for all beam sizes are reported in Table~\ref{table:stats}.
Figure~\ref{figure:plot_5} and Figure~\ref{figure:plot_10} are the $(r_1, r_{2,k})$ scatter plots for $k = 5$ and $k = 10$, respectively.
Looking closely at the statistics and the plots, we have the following observations.
For beam size of 5, the best fit line seems to be flatten and parallel to the x-axis. $|r| < 0.5$ and $R^2 < 0.1$, both indicates a very weak linear correlation between the variables.
For beam size of 10, although both $r$ in absolute value and $R^2$ are larger than in the case of beam size of 5, they are both not significant enough to draw conclusion of strong linear correlation.
In conclusion, we did not see a strong correlation pattern between $r_1$ and $r_{2,k}$ for the case of large beam sizes, specifically, $k = 5$ and $k = 10$.
