# Supplementary material for: Better Language Models of Code through Self-Improvement
Source: arXiv:2304.01228 source file (2023-05-10)
Supplement: Supplementary file 2 [file appendix_c.tex]

\section{Hypothesis on improvement of $\theta_{improved}$}
% The above results align strongly with our hypothesis and expectation from the method.
% Specifically, \textbf{(1)} by fine-tuning the $\theta_{fine-tuned}$ on the pseudo dataset $\tilde{D}$,  we expose the (partial) *pseudo sequence* that model would encounter during inference by training on the model prediction $\hat{y}$, which it will (actually) condition on to generate the next tokens, instead of the ground truth tokens, which is used as the condition in training.
% This helps the model to close the gap between teacher forcing (in training) and non teacher forcing (in inference).
% \textbf{(2)} Since we choose the *pseudo sequence* with high probability through beam search with a large beam size (10 for all tasks in our case), and the model learned on those pseudo sequences, this results in the interpolation of the model to generate the most probable sequence after the self-improving process.
% 
% In other words, from the two of the above statements (1) and (2), the $\theta_{improved}$ learns to replicate the behavior of $\theta_{fine-tuned}$ in finding the high-probability sequences but with less of searching on each generation step, by only using greedy search.
% The table (5) further supports the hypothesis when we compare the sequence probability generated by greedy search of $\theta_{fine-tuned}$ and $\theta_{improved}$, similar to Kim and Rush. This number is averaged over the validation dataset. There is a clear large gap in the probability which showing that the $\theta_{improved}$ learned to output high-probability sequences.
In this section, we give the hypothesis on why $\theta_{improved}$ improves $\theta_{fine-tuned}$ across the beam sizes.

% In summary, the process of generating pseudo data $\tilde{D}$ and fine-tuning $\theta_{fine-tuned}$ on $\tilde{D}$ would benefit the self-improved models through 2 steps
We go through the whole process, generating pseudo data $\tilde{D}$ and fine-tuning $\theta_{fine-tuned}$ on $\tilde{D}$, in a Q\&A way with 2 pairs of question and answer.
\subsection{Q\&A1}
\textbf{Q. What it means to train $\theta_{fine-tuned}$ on pseudo data $\tilde{D}$?}

\textbf{A. Exposing the data distribution of predicted sequences $P_{\theta_{fine-tuned}}(y \mid x)$ to the model.}

In order to solve the generative task, our model is trained in a teacher-forcing manner. In training, model is trained to optimize the loss of the next token given the true-previous tokens.

Specifically, in $i$th training step, we optimize the loss $L$ as a function of model parameters $\theta$
\begin{equation}\label{eq:c1}
		    L(\theta) = -\sum_{j=1}^{V} \log p_{\theta}(t = y_i \mid x, y_{j<i})
\end{equation}
            where:
\begin{itemize}
\item V is the vocabulary size
\item $x$ represents input source sequence
\item $t$ represents current token
\item $y_i$ represents the token at $i$th position in the ground truth sequence $y$
\end{itemize}

However, in inference, at the $i$th inference step, model predicts the next token conditioned on its previous predicted tokens. In other words, it samples the $i$th token from the distribution as the token prediction
\begin{equation}\label{eq:c2}
y_i \sim P_{\theta}(t \mid x, \hat{y}_{j<i})
\end{equation}
where $\hat{y}_{j<i}$ denotes the partial sequence predicted by model.

The major difference lies in the $y_{j<i}$ in Equation~\ref{eq:c1} and $\hat{y}_{j<i}$ in Equation~\ref{eq:c2} as the condition in the probability distribution.

By training on pseudo dataset, the loss is now
\begin{equation}\label{eq:c3}
L(\theta) = -\sum_{j=1}^{V} \log p_{\theta}(t = \tilde{y}_i \mid x, \tilde{y}_{j<i})
\end{equation}
where $\tilde{y}$ is the pseuo target sequence in pseudo data $\tilde{D}$.

Now we condition the distribution on $\tilde{y}$, which is a model prediction. This would expose the model prediction data distribution to $\theta$
\subsection{Q\&A2}
\textbf{Q. Why exposing pseudo data $\tilde{D}$ to $\theta_{fine-tuned}$ improve model performance?}

\textbf{A. Maximizing model likelihood $P_{\theta_{improved}}(y \mid x)$ in greedy search algorithms.}

In this context, we regards greedy search algorithms specifically to beam search algorithms across all beam sizes, not only the case with beam size of 1.

Since $\tilde{y}$ is selected from K-best-list from beam search, $\tilde{y}$ has high mass probability $P_{\theta_{fine-tuned}}(y=\tilde{y} \mid x)$.
By exposing $\tilde{y}$ to $\theta_{improved}$ during improvement-fine-tuning step, the model learns to generate each token, once a step, in a way that, after the generation finished, the predicted sequence will have a very high mass probability. This is done via optimizing $\theta_{fine-tuned}$ on the loss function in Equation~\ref{eq:c3}, in which $\tilde{y}$ appears in the condition.

Eventually, after fine-tuning on $\tilde{D}$, when inferred with greedy search, $\theta_{improved}$ will generate sequences with very high mass probability compared to $\theta_{fine-tuned}$. This is proven empirically in Table~\ref{table:seq_prob}, in which we calculate the average mass probability of predicted sequences with greedy search on both $\theta_{fine-tuned}$ and $\theta_{improved}$. This is also reported by \h{cite the sequence-level distilation paper} in their paper for machine translation problem.
% Close to ground truth

On the otherside, by selecting the pseudo sequence $\tilde{y}$ that close to the ground truth $y$, measured by $sim()$ function, we make sure that the model will not forget the truth data distribution while learning to fit the model generated data distribution $\tilde{D}$.

In conclusion, the performance gain cames from that the $\theta_{improved}$ learned to maximize the likelihood by greedy search algorithms (i.e greedy search and beam search), which leads more probable sequences are generated during inference. This (partially) explained why the method worked.
