# Supplementary material for: Better Language Models of Code through Self-Improvement
Source: arXiv:2304.01228 source file (2023-05-10)
Supplement: Supplementary file 3 [file appendix_single_run.tex]

\section{}
Results for each setting of experiment in this paper are reported with a single run. Note that we kept every hyper-parameters unchanged to the original training script of each model in both fine-tuning and improving stage, including the seed. The only exception is the batch size, and in improving stage, we devide the learning rate by 10 without futher search. So there was no best value of hyper-parameter searched.
